# Supplementary material for: Visual Grounding in Video for Unsupervised Word Translation
Source: arXiv:2003.05078 source file (2020-03-26)
Supplement: Supplementary file 1 [file 06-suppmat-multilingual-compiled.pdf]

## 7.2. Text Evaluation Sets

In this section we provide the full text sets used for our evaluation. The datasets provided are:


7.2.1 Dictionary

7.2.2 Dictionary (Visual)

7.2.3 Simple Words

7.2.4 Simple Words (Visual)

7.2.5 Human Queries


All datasets are available at github.com/gsig/visual-grounding/.

### 7.2.1 Dictionary

The *Dictionary* evaluation set are the "Ground-truth bilingual dictionaries":
en-fr.5000-6500.txt, en-ko.5000-6500.txt, en-ja.5000-6500.txt,
available at github.com/facebookresearch/MUSE.

### 7.2.2 Dictionary (Visual)

Included in the format "EnglishWord FrenchWord" in each line, where each "EnglishWord" can occur in multiple lines (multiple translations). This is a subset of en-fr.5000-6500.txt.

```
torpedo torpille
torpedo torpilles
chat discuter
chat discussion
chat causerie
chat bavardage
chat chat
catholics catholiques
chuck chuck
pit pit
pit fosse
garrison garrison
garrison garnison
sprint sprint
surprised surprise
...
```

Full file: muse_visual_en-fr.5000-6500.txt
Available at github.com/gsig/visual-grounding.

### 7.2.3 Simple Words

Included as "English,French,Korean,Japanese" in each line.

```
a,une,에이,a
able,capable,할 수 있는,できる
about,sur,약,約
absolute,absolu,순수한,絶の
accept,Acceptez,수락,受け入れる
account,Compte,계정,アカウント
achieve,atteindre,이루다,達成する
across,à travers,건너서,に渡って
act,acte,행위,行
active,actif,유효한,アクティブ
actual,réel,실제,際の
add,ajouter,더하다,加える
address,adresse,주소,住所
admit,admettre,들이다,認める
advertise,afficher,공시 하다,告する
...
```

Full file: 1000_most_frequent_en_en_fr_ko_ja.csv
Available at github.com/gsig/visual-grounding.

### 7.2.4 Simple Words (Visual)

Included as "English,French,Korean,Japanese" in each line.

```
across,à travers,건너서,に渡って
afternoon,après midi,대낮,午後
air,air,공기,空
along,le long de,...을 따라서,に沿って
amount,montant,양,量
apart,une part,떨어져서,離れて
apply,appliquer,대다,適用する
area,surface,지역,エリア
arm,bras,팔,腕
around,autour,약...,周り
arrange,organiser,붙이다,アレンジ
art,art,미술,アート
ask,demander,청하다,尋ねる
baby,bébé,아가,赤ちゃん
back,retour,뒤로,バック
...
```

Full file: 1000_most_frequent_en_visual_en_fr_ko_ja.csv
Available at github.com/gsig/visual-grounding.

### 7.2.5 Human Queries

Included as "English,French,Korean,Japanese" in each line.

```
a boy playing,un garçon qui joue,노는 소년,遊んでいる少年
a cartoon animal runs through an ice cave,un animal traverse une grotte de glace dans un dessin animé,
만화 동물은 얼음 동굴을 통해 실행,漫の動物が氷の洞窟をけける
a girl eats ice cream,une fille mange de la glace,여자 아이가 아이스크림을 먹는다,女の子がアイスクリームを食べる
a man driving a red car ,un homme conduit une voiture rouge,빨간 차를 운전하는 사람,赤い車を運する男
a man playing football,un homme jouant au au foot,축구를하는 사람,サッカーをしている男
a man rides a car,Un homme conduit une voiture,한 남자가 차를 타다,男は車にる
a man with a dog,Un homme avec un chien,개를 가진 남자,犬と男
a man withdrawing money from atm,Un homme retire de l'argent d'un distributeur,현금 지급기에서 돈을 인
출 한 사람,ATMからお金を引き出す人
a women wearing red dress,une femme en robe rouge,빨간 옷을 입은 여자,赤いドレスを着ている女性
add pickle,ajoutez des cornichon,피클 추가,漬物を加える
add water,ajoutez de l'eau,물을 더하다,水を加える
air conditionning,Air conditionné,에어컨,エアコン
airplane,avion,비행기,飛行機
alcohol,de l'alcool,알코올,アルコール
animal,animal,동물,動物
...
```

Full file: howto100m_webqueries_clean_en_fr_ko_ja.csv
Available at github.com/gsig/visual-grounding.
